# Supplementary material for: A partially linearized mapping approach to surface hopping (MASH-PLDM) for nonadiabatic dynamics and nonlinear spectroscopy
Source: arXiv:2609.36197 source file (2026-09-28)
Supplement: Supplementary file 1 [file appendix.tex]

Introducing the notation $\hat{V}_k=\hat{V}(q_k)$ and $\hat{W}_k=\nabla\hat{V}(q_k)\cdot\Dq_k$,
\begin{align}
	\hat{T} &= \eu{-i\hat{V}_N\epsilon} \eu{-i\hat{W}_N\epsilon} \eu{-i\hat{V}_{N-1}\epsilon} \cdots \eu{-i\hat{V}_{1}\epsilon} \eu{-i\hat{W}_1\epsilon} \eu{-i\hat{V}_0\epsilon}
	\\
	&= \hat{U} - i \epsilon \sum_{k} \eu{-i\hat{V}_N\epsilon} \eu{-i\hat{V}_{N-1}\epsilon} \cdots \eu{-i\hat{V}_{k+1}\epsilon} \hat{W}_k \eu{-i\hat{V}_k\epsilon} \cdots \eu{-i\hat{V}_{1}\epsilon} \eu{-i\hat{V}_0\epsilon} + \mathcal{O}(t^2)
\end{align}
where we used $\eu{x}=1+x+\mathcal{O}(x^2)$ and we neglect the $\mathcal{O}(N^2)$ terms of order $\mathcal{O}(\epsilon^2)$, which contribute an overall error of $\mathcal{O}(t^2)$.

\begin{align}
	\hat{T} &= \hat{U} - i \epsilon \sum_{k} \int \eu{-i\hat{V}_N\epsilon} \eu{-i\hat{V}_{N-1}\epsilon} \cdots \eu{-i\hat{V}_{k+1}\epsilon} W_k(\S_k) \hat{w}^{-1}(\S_k) \eu{-i\hat{V}_k\epsilon} \cdots \eu{-i\hat{V}_{1}\epsilon} \eu{-i\hat{V}_0\epsilon} \rmd \S_k + \mathcal{O}(t^2)
	\\
	&= \hat{U} - i \epsilon \sum_{k} \int \hat{w}^{-1}(\S_k((N-k)\epsilon)) \eu{-i\hat{V}_N\epsilon} \eu{-i\hat{V}_{N-1}\epsilon} \cdots \eu{-i\hat{V}_{k+1}\epsilon} W_k(\S_k) \eu{-i\hat{V}_k\epsilon} \cdots \eu{-i\hat{V}_{1}\epsilon} \eu{-i\hat{V}_0\epsilon} \rmd \S_k + \mathcal{O}(t^2)
	\\
	&= \hat{U} - i \epsilon \sum_{k} \int \hat{w}^{-1}(\S(N\epsilon)) \eu{-i\hat{V}_N\epsilon} \eu{-i\hat{V}_{N-1}\epsilon} \cdots \eu{-i\hat{V}_{k+1}\epsilon} W_k(\S(k\epsilon)) \eu{-i\hat{V}_k\epsilon} \cdots \eu{-i\hat{V}_{1}\epsilon} \eu{-i\hat{V}_0\epsilon} \rmd \S + \mathcal{O}(t^2)
	\\
	&= \int \hat{w}^{-1}(\S(N\epsilon)) \eu{-i\hat{V}_N\epsilon} \eu{-iW_k(\S((N-1)\epsilon))\epsilon} \eu{-i\hat{V}_{N-1}\epsilon} \cdots \eu{-i\hat{V}_{k+1}\epsilon} \eu{-iW_k(\S(k\epsilon))\epsilon} \eu{-i\hat{V}_k\epsilon} \cdots \eu{-i\hat{V}_{1}\epsilon} \eu{-iW_1(\S(\epsilon))\epsilon} \eu{-i\hat{V}_0\epsilon} \rmd \S + \mathcal{O}(t^2)
\end{align}
because, due to unitary evolution, $\rmd\S = \rmd\S(k\epsilon)$.

The PLDM approach thus captures the QCLE dynamics exactly to first-order in time, but makes an error at longer times.

The error made at second-order in $t$ depends on the mapping scheme.
It is due to terms involving the product of two $\hat{W}$ operators and the difference between the square of the mapped functions.
One hopes that the MASH approach will benefit from the fact that $\sgn(S_z)^2=1$. ???
